# Supplementary material for: TopoBench: Benchmarking LLMs on Hard Topological Reasoning
Source: arXiv:2603.12133 source file (2026-03-12)
Supplement: Supplementary file 1 [file tokens_by_difficulty_appendix.tex]

\clearpage
